# Supplementary material for: Formal Design of Asynchronous Fault Detection and Identification Components using Temporal Epistemic Logic
Source: arXiv:1506.04871 source file (2016-02-10)
Supplement: Supplementary file 1 [file appendix.tex]

\newpage

\section{Proofs}
\subsection{Diagnosability}

\paragraph{Theorem~\ref{th-diagnosable}.}
Let $D$ be a diagnoser for $P$. If $D$ satisfies an alarm
condition $\varphi$ then $\varphi$ is diagnosable in $P$.

\begin{proof}[Theorem~\ref{th-diagnosable}]
By contradiction, suppose $\edel{A}{\beta}{d}$ is not diagnosable in
$P$. Then there exists a critical pair of traces $\sigma_1$ and
$\sigma_2$ such that for some $i\geq 0$ $\sigma_1,i\models\beta$,
$obs(\sigma^{i+d}_1)=obs(\sigma^{i+d}_2)$,
$\sigma_2,i\not\models\beta$. Consider a trace $\sigma$ of the
diagnoser compatible with
$obs(\sigma^{i+d}_1)=obs(\sigma^{i+d}_2)$. If
$\sigma_1\times\sigma\models G(\beta \rightarrow X^n A)$, then
$\sigma_2\times\sigma\not\models G(X^n A\rightarrow\beta)$, which is a
contradiction. If $\sigma_2\times\sigma\models G(X^n
A\rightarrow\beta)$ then $\sigma_1\times\sigma\not\models G(\beta
\rightarrow X^n A)$, which is a contradiction.

Similarly, for $\fdel{A}{\beta}$ and $\bdel{A}{\beta}{d}$.
\end{proof}

\subsection{Maximality and completeness}
\paragraph{Theorem~\ref{thm-max-local-for-completeness}.}
 Given a diagnoser $D$ for a plant $P$ and a \dlocally\ diagnosable
 alarm condition $\varphi$, if $D$ is maximal for $\varphi$ then
 $D$ is complete.

\begin{proof}[Theorem~\ref{thm-max-local-for-completeness}]
Let us denote by $\delta$ and $\delta^{-1}$ respectively the delay
in the future and the delay in the past used in the alarm condition
(thus $\tau=\delta^{-1}\beta$). Suppose $D$ is maximal for $\varphi$
and thus $D\times P\models G(K\delta^{-1}\beta\rightarrow
A_\varphi)$. For all traces $\pi$, for all point $i$, if $\pi,i\models
(\beta\rightarrow \delta K\delta^{-1}\beta)$, then $\pi,i\models
(\beta\rightarrow \delta A)$; thus, $\pi,i\models (\beta\rightarrow
\delta K\delta^{-1}\beta)\rightarrow (\beta\rightarrow \delta A)$.
\end{proof}

\paragraph{Theorem~\ref{thm-max-global-for-completeness}.}
 Given a diagnoser $D$ for a plant $P$ and a \dglobally\ diagnosable
 alarm condition $\varphi$, if $D$ is maximal for $\varphi$ and
 $\varphi$ is diagnosable in $P$ then $D$ is complete.

\begin{proof}[Theorem~\ref{thm-max-global-for-completeness}]
Let us denote by $\delta$ and $\delta^{-1}$ respectively the delay
in the future and the delay in the past used in the alarm condition
(thus $\tau=\delta^{-1}\beta$). Suppose $D$ is maximal for $\varphi$
and $\varphi$ is diagnosable in $P$. Thus $D\times P\models
G(K\delta^{-1}\beta\rightarrow A_\varphi)$ and $P\models
G(\beta\rightarrow \delta K\delta^{-1}\beta)$. For all traces $\pi$,
for all point $i$, if $\pi,i\models \beta$, then by diagnosability
$\pi,i\models \delta K\delta^{-1}\beta$, and by maximality
$\pi,i\models \delta A$. Thus, $\pi,i\models (\beta\rightarrow \delta A)$.
\end{proof}

\subsection{Reachable states of $D \times P$}

\begin{lemma}\label{lem-observations}
For every reachable state $b \times s$ of $ D_\varphi \times P$, for every
trace $\pi$ reaching $b \times s$, for every state $s' \in b$, there
exists a trace $\pi'$ reaching $b \times s'$ with $obs(\pi)=obs(\pi')$.
\end{lemma}

\begin{proof}[Lemma~\ref{lem-observations}]
By induction on $\pi$. If $\pi$ is given by one (initial) state, then
$b\in B_0$ and, by definition of $B_0$, $obs(s)=obs(s')$.  Otherwise,
let $\mktuple{b_1\times s_1, a \times e, b \times s}$ be the last
transition of $\pi$ and let $\pi_1$ the prefix of $\pi$ without this
last transition. For every state $s'\in b$ there exists a transition
$\mktuple{s'_1,e',s'}$ such that $s'_1\in b_1$, $obs(s_1)=obs(s'_1)$,
$obs(e)=obs(e')$, and $obs(s')=obs(s)$. By inductive hypothesis there
exists trace $\pi'_1$ reaching $b_1 \times s'_1$ such that
$obs(\pi_1)=obs(\pi'_1)$. Therefore the concatanation of $\pi'_1$ with
the transition $\mktuple{b_1 \times s'_1, a \times e', b \times s'}$
results in a trace $\pi'$ reaching $b \times s'$ such that
$obs(\pi)=obs(\pi')$.
\end{proof}

\subsection{Synthesis}

\paragraph{Theorem~\ref{th-compatibility}.}
$D_\varphi$ is compatible with $P$.

\begin{proof}[Proof of Theorem~\ref{th-compatibility}]
First note that

\begin{enumerate}
\item For every initial state $s_0$ of $P$, there exists
an initial state $b_0$ of $D_\varphi$ such that $s_0\in b_0$ and
$obs(s_0)\subseteq obs(b_0)$;
\item For every state $b$ of $D_\varphi$, for
every state $s\in b$, for every transition $\mktuple{s,e,s'}$ of $P$,
there exists a transition $\mktuple{b,a,b'}$ of $D_\varphi$ such that
$e\in a$, $s'\in b'$, $obs(e)\subseteq obs(a)$, and $obs(s')\subseteq
obs(b')$;
\item $D_\varphi$ is deterministic;
\item From these three facts, one can prove by induction that if a
state $s\times b$ of the product $P\times D_\varphi$ is reachable,
then $s\in b$.
\end{enumerate}
From 1), 2), 4) it follows that $D_\varphi$ is compatible with $P$.
\end{proof}

\begin{theorem}[Maximality]\label{th-maximality}
$D_\varphi\times P\models G(Kp\rightarrow A_\varphi)$.
\end{theorem}

\begin{proof}[Theorem~\ref{th-maximality}.]
Consider a trace $\pi$ and $i\geq 0$. If $\pi,i\models Kp$, then for
all traces $\pi'$ with $\Obs(\pi)=\Obs(\pi')$, $\pi, i\models p$.  By
lemma~\ref{lem-observations}, all states $s\in \pi[i]$ there exists a
trace $\pi'$ with $\Obs(\pi)=\Obs(\pi')$, and therefore $s\models p$ so
that $\pi[i]\models A_\varphi$.
\end{proof}

\begin{theorem}[Correctness]\label{th-correctness}
$D_\varphi\times P\models G(A_\varphi\rightarrow \tau(\varphi))$.
\end{theorem}

\begin{proof}[Theorem~\ref{th-correctness}]
Consider a trace $\pi$ and $i\geq 0$. Suppose $\pi,i\models A_\varphi$
and let $\pi_{D_\varphi}$ the left component of $\pi$. Then, for all
$s\in \pi_{D_\varphi}[i]$, $s\models p$. Since
$\pi_p[i]\in\pi_{A_\varphi}[i]$ (see proof of
theorem~\ref{th-compatibility}, we can conclude that $\pi_p[i]\models
p$.
\end{proof}

\paragraph{Theorem~\ref{th-ccm} (Correctness, Completeness and Maximality).}
$D_\varphi$ is correct (i.e.\ $D_\varphi\times P\models
  G(A_\varphi\rightarrow \tau(\varphi))$), maximal (i.e.\
  $D_\varphi\times P\models G(Kp\rightarrow A_\varphi)$) and complete
  (under the assumption that if $\varphi$ is \dglobally\ diagnosable,
  then $\varphi$ is diagnosable in $P$).

\begin{proof}[Theorem~\ref{th-ccm}]
Maximality and Correctness follow from Theorems~\ref{th-maximality}
and \ref{th-correctness}. Therefore, we can apply
Theorems~\ref{thm-max-global-for-completeness} or
\ref{thm-max-local-for-completeness} to obtain completeness, depending
on whether $\varphi$ is \dlocally\ diagnosable or
\dglobally\ diagnosable.
\end{proof}

\ignore{
\begin{theorem}
If $\varphi= \edel{A_\varphi}{p}{0}$ and $\varphi$ is diagnosable in $P$,
then $D_\varphi\models\varphi$.
\end{theorem}

\begin{proof}
Given a trace of the product $D_\varphi\times P$ such that $\pi,i\models
p$ for some $i\geq 0$. Let $\pi=\pi_{D_\varphi}\times\pi_P$ for some trace
$\pi_P$ of $P$ and some trace $\pi_{D_\varphi}$ of $D_{\varphi}$. By the
above lemma, for every state $s'\in\pi_{D_\varphi}[i]$, there exists a
trace $\pi'$ reaching $s'\times \pi_{D_\varphi}[i]$ such that
$obs(\pi)=obs(\pi')$. Since $\varphi$ is diagnosable in $P$, then
$\pi',i\models p$, which means that $s'\models p$ and therefore
$b\models A_\varphi$.
\end{proof}}

\paragraph{FiniteDel and BoundDel Relation}
\mg{Lets remove it from the scope of the paper}
\begin{theorem}\label{th-finite-bounded}
Let $P$ be a plant and $p$ be a propositional formula, $\fdel{A}{p}$
is diagnosable in $P$ iff $\exists d.\ \bdel{A}{p}{d}$.
\end{theorem}
\begin{proof}
The key point is that BoundDel requires the existence of a unique
value of $d$ for all traces, while FiniteDel allows for a different
value of $d$ for each trace.
  \begin{itemize}
  \item[$\Leftarrow$] This is the simple case, since FiniteDel is
    $\forall \sigma \exists i$ and BoundDel is $\exists i \forall
    \sigma$, and the second is stronger than the first.
  \item[$\Rightarrow$] Here we need to show that a $d$
    exists. Intuitively, $d$ represents the maximum distance between
    two occurrences of $p$ in all obs-eq traces. ObsEq traces are a
    subset of all possible pair of traces. Therefore, if we show that
    there is a value of $d$ representing the maximum distance between
    two occurrences of $p$ in any two traces, we are done.
\st{This ``we are done'' is not straightforward for me, since it
  requires to consider subtraces that may be not obs equiv.}
    \begin{enumerate}
    \item Lets consider loop-free traces only. Since we are
      considering finite system (and we do not have fairness), there
      is a value $D$ representing the length of the longest path.
      Therefore, we pick $D=d$ and we are done.
    \item For loops we show that we can still compute a $d$ or that
      they make the system not FiniteDel
\begin{itemize}
\item We want to show that if for all $\sigma$ there exists $d$
  s.t. if $\sigma, i \models p$ then $\sigma, j \models p$ for some $j
  \le i+d$.
\item Let $\sigma_1$ and $\sigma_2$ be paths s.t.\ both have a loop
  starting at $i$. We consider $j$ the point in which we leave the
  loop. We need to consider 3 cases:
  \begin{enumerate}
  \item $\sigma_1, j' \models p$ and $\sigma_2, i' \models p$ (for
    $i'\le i$ and $j'\ge j$. This case cannot be FiniteDel diagnosable,
    since for any number of unrolling of $\sigma_1$ we can perform one
    more unrolling in $\sigma_2$, thus increasing the distance between
    the two $p$.
  \item $\sigma_1, k \models p$ and $\sigma_2, i' \models p$ (for $i
    \le k \le j$ and $i'\le i$. In this case, we just need to pick $d
    = k-i'$, to match the first occurrence of $p$ in $k$.
  \item $\sigma_1, j' \models p$ and $\sigma_2, k \models p$ (for $i
    \le k \le j$ and $j \ge j$. In this case, we just need to pick $d
    = j'-k$.
  \end{enumerate}
\end{itemize}

      %% \begin{itemize}
      %%   \item By Observation 2: We know that loops must contain at
      %%     least one observable event. Therefore, a loop leads to
      %%     infinite observable traces. Since our system is finite, the
      %%     only way to have an infinite observable trace is by having a
      %%     loop.
      %% \end{itemize}
      %% Let $\sigma$ be a trace that contains a loop starting at $i$.
      %% \begin{itemize}
      %% \item If the loop does not contain $p$ and $\sigma, j \models p$
      %%   for some $j \le i$ then all traces that are obs-eq up-to $i$
      %%   must contain $p$. Otherwise, we can take the loop forever and
      %%   violate the FiniteDel Diagnosability. (Thus the loop is irrelevant)
      %% \item If the loop contains $p$ then if there is another path
      %%   with a loop starting at $i$ that does not contain $p$, we have
      %%   found a critical pair, and the system was not finitedel
      %%   diagnosable.
      %% \end{itemize}
    \end{enumerate}
  \end{itemize}
\end{proof}
